# Supplementary material for: Scaffolding Sets
Source: arXiv:2111.03135 source file (2021-11-17)
Supplement: Supplementary file 1 [file appendix.tex]

\newpage

\appendix

\noindent\textbf{\Large Appendix}

\section{Proof of Theorem \ref{thm:2vs3}}
\begin{theorem}[Restatement of Theorem \ref{thm:2vs3}]
	There exists a distribution $\cD_x$ for the $d$-dimensional input $x$, and a probability function 
	$$p^*(x)=   \sum_{i=1}^l u^*_i\sigma \left(\sum_{i=1}^l v^*_{i,j}\sigma(w_{i,j}^{*\top} x +b^*_{i,j})+c^*_i\right) $$ 
	such that the following properties hold.
	\begin{itemize}
\item There exists a universal constant $C>0$ such that the following holds. Suppose the input dimension $d>C$, $\alpha >C$ and $N\ge C\alpha^{1.5}d^2$ and let $l$ be an integer satisfying $l\le ce^{cd}$ for a universal constant $c$. There exists a choice of $\epsilon_i \in \{-1,1\}$	such that $p^*(x)$ has the folloiwng property. Let $f$ be any two-layer neural network, \text{i.e.}
$$f(x)=\sum_{i=1}^l v_i\sigma(w_i^\top x +b_i),$$
then, 	
$$\bE_{x\sim \cD_x}|f(x)-p^*(x)|^2\ge \tilde{c}^2/\alpha^2$$
for a universal constant $\tilde{c}$.
	
\item However, if we use our method to build sets upon $\hat{h}$ satisfying learnablility assumption 4 for 
$$h^*=\sum_{j=1}^l v^*_{i,j}\sigma(w_{i,j}^{*\top} x +b^*_{i,j})$$ with $l \le 8c_\sigma/\delta \alpha^{1.5}Nd^3+2$, we can have for any $\hat{p}$ that is $\alpha_n$-multi-calibrated on $\{S^{(\hat{h})}_k\}$,such that $\forall \delta>0$, if sample size $n=\Omega(poly( d,l, N ,1/\delta))$, we have 
$$E_{x}|p^*(x)- \hat{p}(x)|^2\le \delta^2+\alpha_n^2.$$
	\end{itemize}
\end{theorem}

\begin{proof}
We argue by contradiction. Consider $\tilde{g}(x)$ defined in \cite{xx}. For the function $\tilde{g}$, it has the following properties: there exists a distribution $\cD_x$, such that

\begin{itemize}
    \item $\tilde{g}(x)\in [-1,1]$.
    \item   There exists a universal constant $C>0$ such that the following holds. Suppose the input dimension $d>C$, $\alpha >C$ and let $l$ be an integer satisfying $l\le ce^{cd}$ for a universal constant $c$. Let $f$ be any two-layer neural network, \text{i.e.}
$$f(x)=\sum_{i=1}^l v_i\sigma(w_i^\top x +b_i),$$
then, 	
$$\bE_{x\sim \cD_x}|f(x)-\tilde{g}(x)|^2\ge \tilde{c}^2/\alpha^2$$
for a universal constant $\tilde{c}$.
\item There exists a universal constant $C>0$ such that the following holds. Suppose the input dimension $d>C$, $\alpha >C$, there exists a three-layer neural network $g$, \textit{i.e.}
$$g(x)= \sum_{i=1}^l u_i\sigma \left(\sum_{j=1}^l v_{i,j}\sigma(w_{i,j}^\top x +b_{i,j})+c_i\right )$$
with width at most $8c_\sigma C/\delta \alpha^{3}d^5+1$ for a universal constant $c_\sigma$ such that 
$$\bE_{x\sim \cD_x}|\tilde{g}(x)-g(x)|^2\le (\frac{\sqrt{3}}{\alpha d^{0.25}}+\delta)^2.$$
\end{itemize}

Note that $\tilde{g}$ already is bounded in $[-1,1]$, thus we only need to prove that $\frac{1}{2}\tilde{g}+\frac{1}{2}$ shares the same properties as $\tilde{g}$, then we can take $$p^*=\frac{1}{2}\tilde{g}+\frac{1}{2}$$

since $\frac{1}{2}\tilde{g}+\frac{1}{2}\in [0,1]$.

We first claim that for $p^*=\frac{1}{2}\tilde{g}+\frac{1}{2}$, there exists a universal constant $C>0$ such that the following holds. Suppose the input dimension $d>C$, $\alpha >C$ and let $l$ be an integer satisfying $l\le ce^{cd}$ for a universal constant $c$. Let $f$ be any two-layer neural network, \text{i.e.}
$$f(x)=\sum_{i=1}^l v_i\sigma(w_i^\top x +b_i),$$
then, 	
$$\bE_{x\sim \cD_x}|f(x)-p^*(x)|^2\ge \tilde{c}^2/\alpha^2$$
for a universal constant $\tilde{c}$.

If not, for any $\varepsilon>0$, there exists a two-layer neural network $f_{\varepsilon}$ with $l\le ce^{cd}$, such that 

$$\bE_{x\sim \cD_x}|f_\varepsilon(x)-p^*(x)|^2\le \varepsilon^2.$$

Then, there must exist $f'_{\varepsilon}(x)$ with width at most $ce^{cd}+1$ such that 

$$\bE_{x\sim \cD_x}|f'_\varepsilon(x)-\tilde{g}(x)|^2\le 4\varepsilon^2,$$

since we can rescale the weights and bias and add at most one node to obtain $f'_\varepsilon(x)=2f_{\varepsilon}(x)-1$. Thus, for any $\varepsilon>0$, there exists a universal constant $C>0$ such that the following holds. Suppose the input dimension $d>C$, $\alpha >C$ and let $l$ be an integer satisfying $l\le 2ce^{2cd}$ for a universal constant $c$. there exists $f'_\varepsilon$, \text{i.e.}
$$\bE_{x\sim \cD_x}|f'_\varepsilon(x)-\tilde{g}(x)|^2\le 4\varepsilon^2,$$

which contradicts.

Secondly, notice we only need to add one extra node for the three-layer neural network and rescale the weights and bias so that there exists a universal constant $C>0$ such that the following holds. Suppose the input dimension $d>C$, $\alpha >C$, there exists a three-layer neural network $g'$, 
with width at most $8c_\sigma C/\delta \alpha^{3}d^5+2$ for a universal constant $c_\sigma$ such that 
$$\bE_{x\sim \cD_x}|\tilde{g}(x)-g'(x)|^2\le (\frac{\sqrt{3}}{\alpha d^{0.25}}+\delta)^2.$$
The proof is complete.

\end{proof}

\newpage

\textbf{Old Proof}

%\iffalse

Let us briefly introduce the structure of neural networks we consider in this paper. We consider the input with dimension $d$.
\begin{itemize}

\item Two-layer neural network:

$$x\mapsto \sum_{i=1}^l v_i\sigma(w_i^\top x +b_i)$$

where $v_i\in \bR$ and $w_i \in \bR^d$.

\item Three-layer neural network:
$$x\mapsto  \sum_{i=1}^l u_i\sigma \left(\sum_{j=1}^l v_{i,j}\sigma(w_{i,j}^\top x +b_{i,j})+c_i\right )$$

\end{itemize}
In this section, we only consider $\sigma$ is the ReLU function.
\subsection{Notations}

Let $B_d$ to be the $d-dimensional$ ball with radius $1$ and center  $0$. Let $R_d$ to be $\sqrt{1/\pi}(\Gamma(d/2+1))^{1/d}$. Thus, $R_dB_d$ will have volume $1$. For function $f$, $g$, $\langle f,g\rangle_{L_2}=\int f(x)g(x)dx$ and $\langle f,g\rangle_{L_2(\mu)}=\int f(x)g(x)d\mu(x)$. The corresponding norm induced by the inner product are $\|\cdot\|_{L_2}$ and $\|\cdot\|_{L_2(\mu)}$ respectively.

\paragraph{Fourier Transformation} For a function $f:\bR^d\mapsto\bR$, let us denote the fourier transformation to be 
$$\hat{f}(w)=\int _{\bR^d}\exp(-2\pi i \langle w,x\rangle)f(x)dx.$$

\paragraph{Construction of Hard to Get Functions} To define the hard to approximate functions, we introduce some notations, Let $\alpha\ge 1$ and $\gamma$ be some large numerical constant to be determined later. Then, let $N=\gamma d^2$ and assumed to be an integer. Consider the intervals:

$$\Delta_i=[(1+\frac{i-1}{N})\alpha\sqrt{d},  1+\frac{i}{N})\alpha\sqrt{d}],~i=1,2,\cdots,N.$$

We say that  interval $\Delta_i$ is good (or simply say $i$ is good) if for any $x\in \Delta_i$
$$J^2_{d/2}(2\pi R_dx)\ge \frac{1}{80\pi R_d x},$$
where $J$ is the Bessel function. Otherwise, we say $\Delta_i$ is bad.

Then, we define $g_i$ such that $g_i(\|x\|)=1\{\|x\|\in\Delta_i\}$ if $i$ is good, and $g_i(x)=0$ if $i$ is bad.

We further define 
$$\psi(x) = (R_d/\|x\|)^{d/2}J_{d/2}(2\pi R_d\|x\|).$$

In this section, we consider $x$ follows the probability measure $\mu$ with density function  $\psi^2(x)$.

\begin{lemma}\label{lm:1}
 Let 
$$\rho_i (x)=\frac{1+3\epsilon_i}{4}g_i(\|x\|) $$
where $\epsilon_i \in \{-1,1\}$. 

There is a choice of $\epsilon_i \in \{-1,1\}$, $i=1,\cdots,N$ such that 

$$\int_{\bR^d\backslash(2R_dB_d)}[\widehat{(\sum_{i=1}^N \epsilon_i\rho_i\psi)}(w)]^2dw \ge c$$
where $c$ is a universal constant.

\end{lemma}

\begin{proof}
Let us randomly choose $\epsilon_i$  from $\{-1,1\}$ indepedently. It suffices to show that 

$$\bE \int_{\bR^d\backslash(2R_dB_d)}[\widehat{(\sum_{i=1}^N \epsilon_i\rho_i\psi)}(w)]^2dw \ge c$$
where $c$ is a universal constant.

\begin{align*}
\bE \int_{\bR^d\backslash(2R_dB_d)}[\widehat{(\sum_{i=1}^N \epsilon_i\rho_i\psi)}(w)]^2dw &=\frac{1}{16}\bE \int_{\bR^d\backslash(2R_dB_d)}[\widehat{(\sum_{i=1}^N \epsilon_ig_i\psi)}(w)]^2dw\\
&+\frac{3}{8}\bE \int_{\bR^d\backslash(2R_dB_d)}[\widehat{(\sum_{i=1}^N \epsilon_ig_i\psi)}(w)](\sum_{i=1}^N\widehat{g_i\psi}(w))dw\\
&+\frac{9}{16}\bE \int_{\bR^d\backslash(2R_dB_d)}[\sum_{i=1}^N\widehat{g_i\psi}(w)]^2dw
\end{align*}                                                                     

The second term is $0$ and the last term is positive, the first term is lower bounded by some universal $c$ by Lemma 8 in \cite{xx}. The proof is complete.

\end{proof}

Next, we provide a lemma to show that the linear combination $\epsilon_i\rho_i$ has a non-negligible mass under $L_2$ distance  and density function $\psi^2(x)$.

\begin{lemma}\label{lm:2}
Suppose $\alpha\ge c$, $N\ge c(\alpha d)^{3/2}$	for some sufficiently large universal constant $c$, then for every choice of $\epsilon_i\in\{-1,1\}$, $i=1,2,\cdots, N$, one has
	
$$\int\Big(\sum_{i=1}^N\epsilon_i\rho_i(x)\Big)^2\psi^2(x)dx\ge \frac{0.00075}{\alpha}.$$	
\end{lemma}

\begin{proof}
Since $g_i$ has disjoint support for different $i$, we have

\begin{align*}
\int\Big(\sum_{i=1}^N\epsilon_i\rho_i(x)\Big)^2\psi^2(x)dx&=\int\Big(\sum_{i=1}^N\frac{\epsilon_i+3}{4} g_i(\|x\|)\Big)^2\psi^2(x)dx\\
&=\sum_{i=1}^N\int\Big(\frac{\epsilon_i+3}{4} g_i(\|x\|)\Big)^2\psi^2(x)dx\\
&\ge \sum_{i=1}^N\frac{1}{4}\int\Big( g_i(\|x\|)\Big)^2\psi^2(x)dx.
\end{align*}
Then, by Lemma 6 in \cite{xx}, we have 
$$\sum_{i=1}^N\frac{1}{4}\int\Big( g_i(\|x\|)\Big)^2\psi^2(x)dx\ge \frac{1}{4}\frac{0.003}{\alpha}=\frac{0.00075}{\alpha}.$$
\end{proof}

\paragraph{Inapproximability of the two-layer neural networks.} We consider the probability function:
$$p^*(x)=\sum_i \epsilon_ig_i(\|x\|)$$
where $\{\epsilon_i\}_i$ are the signs provided by Lemma \ref{lm:1}.

\begin{theorem}
There exists a universal constant $C>0$ such that the following holds. Suppose the input dimension $d>C$, $\alpha >C$ and $N\ge C\alpha^{1.5}d^2$ and let $l$ be an integer satisfying $l\le ce^{cd}$ for a universal constant $c$. There exists a choice of $\epsilon_i \in \{-1,1\}$	such that $p^*(x)$ has the folloiwng property. Let $f$ be any two-layer neural network, \text{i.e.}
$$f(x)=\sum_{i=1}^l v_i\sigma(w_i^\top x +b_i),$$
then, 	
$$\|f-p^*\|_{L_2(\mu)}\ge \tilde{c}/\alpha$$
for a universal constant $\tilde{c}$.

\end{theorem}

\begin{proof}

According to Lemma \ref{lm:2}, we know that 
$$\|p^*\|_{L_2(\mu)}\ge \frac{c_1}{\alpha},$$
where $\|\cdot\|_{L_2(\mu)}$ is the $L_2$ norm under probability measure $\mu$ and $c_1$ is a universal constant $c_1>0$. Note that the function $|p^*(x)|\le 1 $ for any $x$, and define $w=\widehat{p^*\psi}/\|p^*\psi\|_{L_2}$.

\begin{align*}
\int_{2R_dB_d}w(x)^2dx&=1-\frac{\int_{2R_dB_d}\widehat{p^*\psi}(x)^2dx}{\|p^*\psi\|^2_{L_2}}\\
&\le 1-\frac{\int_{2R_dB_d}\widehat{p^*\psi}(x)^2dx}{\|\psi\|^2_{L_2}}\\
&\le 1-c_2
\end{align*}
for a universal constant $c_2>0$ and the first inequality is due to $|p^*(x)|\le 1$ for all $x$ and the second one is due to Lemma \ref{lm:1}.

Next, for any two-layer neural network $f$, \textit{i.e.}
$$f(x)=\sum_{i=1}^l v_i\sigma(w_i^\top x +b_i),$$

we define $q=\widehat{f\psi}/\|f\psi\|_{L_2}$. By Claim $2$  and Lemma $9$ in \cite{xx}, we have
$$\langle q,w\rangle_{L_2}\le 1-c_2/2+l\exp(-c_3d)$$
for a universal constant $c_3>0$. Besides,  given $\|q\|_{L_2}=\|w\|_{L_2}=1$,  by Proposition $1$ in \cite{xx}, we have for every scalars $\beta_1,\beta_2>0$ that
$$\|\beta_1 q - \beta_2 w\|_{L_2}\ge \frac{\beta_2}{2}\|q-w\|_{L_2}.$$

As a result, 
\begin{align*}
\|f-p^*\|_{L_2(\mu)}&=\|f\psi-p^*\psi\|_{L_2}=\|\|f\psi\|_{L_2}q(\cdot)-\|p^*\psi\|_{L_2}w(\cdot)\|_{L_2}\\
&\ge \frac{1}{2}\|q-w\|_{L_2}\|p^*\|_{L_2(\mu)}\\
&\ge \frac{1}{2}\sqrt{2(1-\langle q,w \rangle_{L_2} )} \frac{c_1}{\alpha}\\
&\ge \frac{c_1}{2\alpha} \sqrt{2\max (c_2/2-l\exp(-c_3d),0)}\ge \frac{c_1\sqrt{c_2}}{4\alpha}.
\end{align*}
The last inequality follows if we take $c=\min\{c_2/4,c_3\}$.
\end{proof}

\paragraph{Approximability of the three-layer neural networks.}

\begin{theorem}
There exists a universal constant $C>0$ such that the following holds. Let $\delta\in(0,1)$. Suppose that $d\ge C$ and for any choice of $\epsilon\in\{-1,1\}$, $i=1,\cdots, N$ there exists a three-layer neural network 
$$g= \sum_{i=1}^l u_i\sigma \left(\sum_{i=1}^l v_{i,j}\sigma(w_{i,j}^\top x +b_{i,j})+c_i\right )$$
with $l \le 8c_\sigma/\delta \alpha^{1.5}Nd^3+2$ for some universal constant $c_\sigma$, such that 
$$\|g(x)-\sum_{i=1}^N \epsilon_i\rho_i(\|x\|)\|_{L_2(\mu)}\le \frac{\sqrt{3}}{\alpha d^{0.25}}+\delta.$$
Moreover, $g$ is $L$-Lipchisz constant, where $L=O(poly(d,N,1/\delta))$.
\end{theorem}

\begin{proof}
Note that $\sum_{i=1}^N \epsilon_i\rho_i(\|x\|)$ is just a linear transformation of $ \sum_{i=1}^N \epsilon_ig_i(\|x\|)$, we at most need add one more note to approximate $\sum_{i=1}^N \epsilon_i\rho_i(\|x\|)$. Other part follows exactly the same as Proposition $2$ in \cite{xx}.

\end{proof}
%\fi
